# Supplementary material for: Dyn-E: Local Appearance Editing of Dynamic Neural Radiance Fields
Source: arXiv:2307.12909 source file (2025-04-12)
Supplement: Supplementary file 1 [file 06_supp.tex]

Our supplementary material includes information on network architectures, training details, additional experimental results, and discussions.
\section{network architectures}
\subsection{Invertible Networks}
%网络结果和CaDeX的'nvp_v2'的网络架构相同。我们采用了他官方的实现,
The architecture of our invertible networks is the same as the ``NVP'' in CaDeX~\cite{Lei2022CaDeX}.

\subsection{Scene Flow Fields}
\input{contents/network/MLP}
We show the architectures of the scenes flow fields $f_\phi$ in~\figref{mlp}.
% 在每个layer后会接着一个激活层ReLU，除了最后一层
We add a ReLU activation after each layer except the last layer.
\input{contents/nerf_baseline/nerf_baseline.tex}
\section{Training details}
%预先处理编辑的图片
\subsection{Preprocessing of the Edited Image}
%在训练之前我们会对编辑的图片进行预处理。
Before training, we will preprocess the edited image.
% 我们一般会把reference图片的编辑区域的最小包围盒作为需要提升到3D的区域。
We usually take the minimum bounding box of the edited area of the reference image as the area that needs to be lifted to 3D.
% 这是因为如果我们对编辑的效果不满意，我们只需要挑选一个小于这个包围盒的纹理重新编辑即可。
This is because if we are not satisfied with the edited results, we only need to select a texture smaller than this bounding box to edit the reference image again. 
%  这样我们就可以重复利用训练好的模型，而不需要重新训练。
In this way, we can reuse the trained model.
% 编辑后，渲染的时候，我们对于在编辑区域之外的点但在包围盒内的点，我们会把它们的透明度设置为0，并且把opacity信息也作为mesh顶点的一个属性。
When rendering, for points outside the edited area but inside the bounding box, we will set their opacity to 0, and the opacity information is also used as an attribute of the mesh vertices.
% 我们可以通过mesh renderer很容易的得到其他视角的opacity信息。
We can easily render the opacity values at other views 
through the mesh renderer.
% 对于opacity等于0的ray，我们将rays上面的local surface的density设置为0。
For rays with opacity equal to 0, we set the density of the local surface along the rays to 0.

\subsection{Loss Functions}
To train our scenes flow fields $f_\phi$, we use the same loss function as in~\cite{Gao2021DynNeRF},
including motion regularization, cycle consistency, dynamic rendering photo-metric loss
, and motion matching loss.
We apply motion regularization to encourage the scene flow to be slow and temporally smooth:
\begin{equation}
\begin{aligned}
\mathcal{L}_{slow} & =\sum_{\mathbf{r}\in \mathcal{R}}\left\|\mathbf{f}_{t \rightarrow t+1}\right\|_1+\left\|\mathbf{f}_{t \rightarrow t-1}\right\|_1 \\ 
\mathcal{L}_{smooth} & =\sum_{\mathbf{r}\in \mathcal{R}}\left\|\mathbf{f}_{t \rightarrow t+1} + \mathbf{f}_{t \rightarrow t-1}\right\|_2^2.
\end{aligned}
\end{equation}
The cycle consistency loss is 
\begin{equation}
\begin{aligned}
\mathcal{L}_{cycle} & =\sum_{\mathbf{r}\in \mathcal{R}}\left\|\mathbf{f}_{t \rightarrow t+1} +\mathbf{f}_{t+1 \rightarrow t}\right\|_2^2+\left\|\mathbf{f}_{t \rightarrow t-1} +\mathbf{f}_{t-1 \rightarrow t}\right\|_2^2.
\end{aligned}
\end{equation}
The dynamic rendering photometric loss is defined as:
\begin{equation}
\begin{aligned}
\mathcal{L}_{pho}=\sum_{\mathbf{r}_i} \sum_{j \in\{i \pm 1\}}\left\|\hat{\mathbf{C}}_{j \rightarrow i}\left(\mathbf{r}_i\right)-\mathbf{C}_i\left(\mathbf{r}_i\right)\right\|_2^2,
\end{aligned}
\end{equation}
where $\hat{\mathbf{C}}_{j \rightarrow i}$ is the color of the pixel $\mathbf{r}_i$ rendered from the view $j$ and warped by the scene flow field $\mathbf{f}_{j \rightarrow i}$.
$\mathbf{C}_i$ is the color of the pixel $\mathbf{r}_i$ in the view $i$.
The motion matching loss is introduced in the main paper.
The overall loss function is:
\begin{equation}
\begin{aligned}
\mathcal{L}_{flow}=\lambda_1 \mathcal{L}_{slow}+\lambda_2 \mathcal{L}_{smooth}+\lambda_3 \mathcal{L}_{cycle}\\+\lambda_4 \mathcal{L}_{pho}+ \lambda_5 \mathcal{L}_{motion},
\end{aligned}
\end{equation}
where $\lambda_1 = 0.01$, $\lambda_2 = 0.1$, $\lambda_3 = 1.0$, $\lambda_4 = 1$, and $\lambda_5 = 0.02$.

To train our invertible networks, we use distillation loss, Laplacian smooth regularization, feature-based photometric term, surface position regularization, and depth consistency loss.

The distillation loss $\mathcal{L}_{distill}$, Laplacian smooth regularization $\mathcal{L}_{lap}$, and feature-based photometric term $\mathcal{L}_{pho}$ are introduced in the main paper.
We add surface motion regularization $\mathcal{L}_{surf}$ to constrain the motion of local surface position from frame $i$ to $i \pm 1$ be consistent with the ground truth optical flow from frame $i$ to $i \pm 1$.
% % 注意我们只对可见的顶点加这个约束，如公式：
Note that we only add this constraint to the visible vertices, as shown in~\equref{optical_flow_consistency}:
\begin{equation}
\mathcal{L}^t_{opt}=\sum_{k=1}^{K}\sum_{j \in\{i \pm 1\}}||\hat{\mathbf{p}}^k_{i \rightarrow j} - \Pi({\mathbf{m}}^k_{i \rightarrow j})||,
\label{optical_flow_consistency}
\end{equation}
where $\hat{\mathbf{p}}^k_{i \rightarrow j}$ is the ground truth  optical flow from frame $i$ to $j$. $K$ is the number of mesh vertices. $\Pi(\cdot)$ is the projection function. $\mathbf{m}^k_{i \rightarrow j}$ is the moiton of $k$-th vertex $\mathbf{v}^k_i$ from frame $i$ to $j$.
% 我们还加了一个depth consistency loss，如公式：
We also add a depth consistency loss to constrain the depth values of the local surface to be consistent with the depth values of the given dynamic NeRFs.
% 注意我们只对可见的顶点加这个约束，如公式：
Note that we only add this constraint to the visible vertices, as shown in~\equref{depth_consistency}:
\begin{equation}
\mathcal{L}^t_{depth}=\sum_{\mathbf{v}^i_t \in \mathcal{V}^t_{vis}}||\hat{d}^i_{t} - d^i_{t}||,
\label{depth_consistency}
\end{equation}
where $\hat{d}^i_{t}$ is the depth value 
projected from the 3D position of the
vertex $\mathbf{v}^i_t$. $d^i_{t}$ is the depth value of the given dynamic NeRFs at the corresponding pixel. $\mathcal{V}^t_{vis}$ is the set of visible vertices at frame $t$. 
The overall loss functions for training the invertible networks are:
\begin{equation}
\begin{aligned}
\mathcal{L}_{inv}=\lambda_6 \mathcal{L}_{distill}+\lambda_7 \mathcal{L}_{lap}+\lambda_8 \mathcal{L}_{pho}+\lambda_9 \mathcal{L}_{surf}+\lambda_{10} \mathcal{L}_{depth},
\end{aligned}
\end{equation}
where $\lambda_6 = 1.0$, $\lambda_7 = 0.001$, $\lambda_8 = 0.01$, $\lambda_9 = 0.02$, and $\lambda_{10} = 0.1$.
The total loss function for training our framework is:
\begin{equation}
\begin{aligned}
\mathcal{L}_{total}= \mathcal{L}_{flow}+\mathcal{L}_{inv},
\end{aligned}
\end{equation}
\input{contents/beta_gamma/betagamma.tex}
\input{contents/alternative/alternative.tex}

\section{additional experimental results}

\paragraph{Artifacts of the naive baseline.}
% 我们另一个重要的component是local surface，我们设计了一个些naive surface alternatives来验证我们的local surface的有效性。
We design several naive alternatives to verify the effectiveness of our framework.
% 我们使用了``curls''这个在Nerfies数据集里的数据，我们使用Nerfies建模整个动态场景。
We utilize the ``curls'' scene in the Nerfies dataset to conduct our experiments.
% The Nerfies is trained to model this dynamic scene, and a single  image被编辑去修改nerfies。
The Nerfies is trained to model this dynamic scene, 
and a single image is edited to modify the Nerfies.
% 第一，为了验证直接在单张编辑图片上面finetune NeRF会造成overfit的问题，
% 训练好的Nerfies被用来在单张编辑图片上面finetune。
To verify that fine-tuning NeRF on a single edited image will cause the overfitting problem,
the Nerfies is used to fine-tune on a single edited image.
% 我们只训练建模canonical space的MLP，其他网络参数全部被冻住
We only train the MLP that models the canonical space and freeze all other network parameters.
% 图~\todo{fig}展示了finetune过后的在fixed time novel view的结果。
\figref{baseline} shows the rendered results of the fine-tuned model at the novel view of the same time step as the reference image.
% There are 许多空中的floating 噪声,编辑的图案在其他视角呈现了blur和扭曲的artifact。
There are many floating noises in the air, and the edited region presents blurred and distorted artifacts at novel views.

%rewrite "There are many floating noises in the air, and the edited region presents blur and distorted artifacts at novel views.":
%

\paragraph{Compared with the alternative of motion representation.}
The alternative to motion representation is to use an MLP to model the motion of each vertex of the local surface.
%我们只在mesh vertices加scene flows的监督
The supervision of scene flows is only added to the mesh vertices.
%其余pipeline和我们的方法一样
The rest of the pipeline is the same as our method.
%然而我们发现这个alternative效果并不好，如图~\todo{fig}所示。
However, we find that the temporal consistency of this alternative is not satisfactory. As shown in~\figref{alternative}, its edited results tend to be distorted.

\paragraph{Impact of $\beta$ and $\gamma$ values.}
%我们发现调节$\beta$和$\gamma$的值不太会影响结果，我们的方法对这两个比较鲁棒。
Our method is robust to $\beta$ and $\gamma$ values.
%对于一个被scale在[-1,1]的场景，我们经验上设置$\beta=0.001$和$\gamma=\beta$  
For a scene scaled in [-1,1], we empirically set $\beta=0.001$ and $\gamma=\beta$.
We show the rendered results of different $\beta$ and $\gamma$ values in~\figref{gamma}

% mask field的重要性
\paragraph{Importance of the mask field.}
% 我们的方法的一个重要component是mask field，我们设计了一个没有mask field的alternative来验证我们的mask field的有效性。
An important component of our method is the mask field. 
We design an alternative without the mask field to verify the effectiveness of our mask field.
As shown in~\figref{mask}, the alternative without the mask field presents obvious artifacts at the edited region, 
% 因为原来的dynamic NeRFs会盖住local surface
because the original dynamic NeRFs will cover the local surface.
\input{contents/maskfield/maskfield.tex}
\section{disscusssion}
%depth map的质量的影响
\subsection{Impact of the Quality of Depth Map}
% 值得讨论的是，我们的方法需要用到dynamic NeRFs的渲染得到的depth map。
It is worth noting that our method requires the depth map rendered by the dynamic NeRFs.
% 但这不意味着dynamic NeRFs的渲染得到的depth map需要和真实的depth map一样精确。
However, this does not mean that the depth map rendered by the dynamic NeRFs 
needs to be as accurate as the ground truth depth map. 
% 我们的方法相当于在dynamic NeRFs的表面上贴上一层layer。
Our method is able to be interpreted as a layer attached to the surface of the dynamic NeRFs.
% 因此只需要保证我们的layer和dynamic NeRFs的表面重合就可以了。
Thus, our local surface only needs to ensure that it overlaps with the surface of the dynamic NeRFs.

\subsection{SDF-based Method}
% 现有有一些方法将SDF-based的方法~\cite{yariv2021volume,wang2021neus}拓展到动态场景上。
Existing methods~\cite{Cai2022NDR,qiao2022neuphysics,johnson2023ub4d} extend the SDF-based~\cite{yariv2021volume,wang2021neus} representations to dynamic scenes. However, 
% 他们只展示了结果在简单的场竞上，或者有RGBD数据的情况下
they only show the results on simple scenes or RGBD datasets.
%现在主流的dynamic view生成的方法是NeRF-based的方法，因为SDF-based的方法专注于提升几何效果，并没有和NeRF-based的方法比较渲染效果。
Additionally, the current mainstream dynamic view synthesis methods are NeRF-based methods,
because the SDF-based methods focus on improving the reconstruction performance and do not compare the rendering performance with NeRF-based methods.
%我们method可以和大部分主流算法结合，因此不编辑的渲染质量可以和主流算法一致
Our method can be combined with most dynamic view synthesis methods,
so the rendering quality of the unedited region is consistent with the mainstream algorithms.
% 's rendering performance tends to be worse than NeRF when they are used to model dynamic scenes.  
% We directly replace the density representation of Nerfies with SDF-induced density.
% 然后我们利用SDF场提取每一帧的mesh，这样就可以比我们的方法获得更加完整的surface了
% Unfortunately, due to the complexity of the dynamic scene, the SDF-based method fails to produce high-quality results.
\subsection{Limitations}
% 对于拓扑变化比较大的情况，我们的方法不能处理。
Our method cannot handle large topological changes, as shown in~\figref{fail}.
% 当optical flow完全fail的时候，我们的方法也会fail
Additionally, when the optical flow estimation network
 fails, our method also fails.
 \begin{figure*}[htbp]
\begin{center}
\setlength\tabcolsep{0.2em}
\newcommand{\mywidth}{0.5 \textwidth}
\begin{tabular}{cc}
\includegraphics[width=\mywidth]{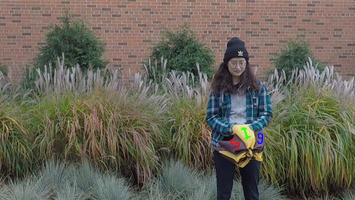}
&\includegraphics[width=\mywidth]{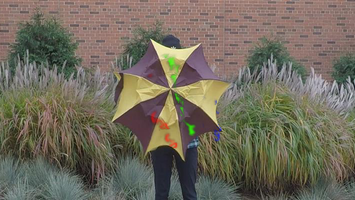}

\\
Input edited image
&
Other frame
\end{tabular}
\end{center}
\vspace{-0.2em}
\captionsetup{font={normalsize}} 
\caption{\textbf{Failure case.}
Our method fails when the topological change is too large.}

\vspace{-1em}

\label{fail}
\end{figure*}
